# Supplementary material for: Strong Pressure Dependent Electron-Phonon Coupling in FeSe
Source: arXiv:1401.3782 source file (2014-01-15)
Supplement: Supplementary file 1 [file Supplementray.pdf]

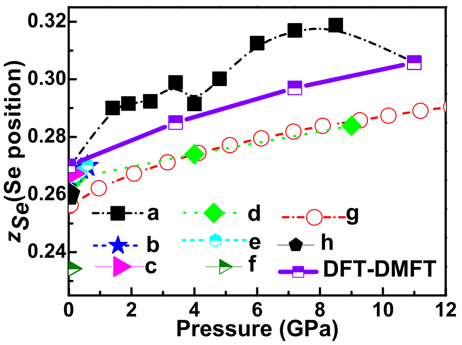


FIG. 1. (Color online). Pressure dependence of chalcogen position parameter $z_{Se}$. a, b, and c are the experimental data of $z_{Se}$ for the tetragonal phase, obtained from Ref.[6], Ref.[8], and Ref.[9] respectively; d and e are the data for the low temperature orthorhombic phase, obtained form Ref. [10] and Ref. [8] respectively. f (Ref. [11]), g(Ref. [12]) indicates non-spinpolarized DFT results and h indicates our spin-polarized DFT results of $z_{Se}$ while the solid line refers to DFT-DMFT.

## SUPPLEMENTARY METHODS

In the DFT-DMFT method, the self-energy, sampling all Feynman diagrams local to the Fe ion, is added to the DFT Kohn-Sham Hamiltonian[1, 2]. This implementation is fully self-consistent and all-electron [2, 3]. The computations are converged with respect to charge density, impurity level, chemical potential, self-energy, lattice and impurity Green's functions. The lattice is represented using the full potential linear augmented plane wave method, implemented in Wien2k[4] package in its generalized gradient approximation (PBE-GGA). We use the continuous time quantum Monte Carlo method to solve the quantum impurity problem and to obtain the local self-energy due to the correlated Fe 3d orbitals. The self-energy is analytically continued from the imaginary to real axis using an auxiliary Green's function. We fixed the Coulomb interaction $U$ and Hund's coupling $J$ at 5.0 eV and 0.7 eV, respectively [5]. We used a fine k-point mesh of $24 \times 24 \times 16$ and 80 million Monte Carlo steps for each iteration for the paramagnetic phase of the FeSe at room temperature within the pressure range of 0-11 GPa where FeSe is observed to remain in its tetragonal phase[6]. The lattice parameters are obtained from the experiment[6] and $z_{Se}$ are optimized within DFT-DMFT method. For P=-2GPa, we estimated the lattice parameters and $z_{Se}$ after fitting. The estimated lattice parameters for -2GPa are a=3.82178 $\mathring{A}$, c=5.7119$\mathring{A}$, and $z_{Se} = 0.25872$.

## DEFORMATION POTENTIAL

The shift in the energy eigenvalues at $E_F$ due to a particular phonon mode is calculated by:$\delta E = 1/N_{kF} \sum_{kF} (E_{kF} - E_{kF}^{A1g})$. Here $E_{kF}$ and $E_{kF}^{A1g}$ are the energy eigenvalues around the Fermi level respectively for equilibrium and $A_{1g}$ distortion. Here $E_{kF}$ is the band resolved energy eigenvalues for the equilibrium structure, chosen within a very small energy window of 5 mRy around $E_F$ within a fine k-point mesh of 25x25x17 to allow at least $\sim$ 2000 points on the FS for each pressure. $E_{kF}^{A1g}$ is the corresponding energy eigenvalues to the $A_{1g}$ distortion. Equilibrium position is where the total energy is minimum in the respective methods whereas $A_{1g}$ distortion refers to the states with small Se atom displacement ($Q$) in the $z_{Se}$. $N_{kF}$ is the number of k-points (kF) on the Fermi surface on which the deformation potential ($\mathcal{D} = \frac{\delta E}{\delta Q}$) is calculated. $\lambda$ is then estimated as $\frac{\mathcal{D}^2}{\frac{\delta^2 E_t(Q)}{\delta Q^2}|_{Q=0}}$, where $E_t(Q)$ is the total energy as a function of the atomic displacement Q in the DFT-DMFT frozen-phonon calculation [7].

In Table I $\mathcal{D}^m$, $\mathcal{D}^{avg}$, $N_{kF}$, and $\mathcal{D}_{FS}^{avg}$ refer to the maximum deformation potential, deformation potential averaged over corresponding pocket, number of k-points on the pocket, and deformation potential averaged over all available pockets (averaged over the entire Fermi surface) respectively. h1, h2, h3, e1, and e2 are labeled in Fig. 1(d-f) in the main text.

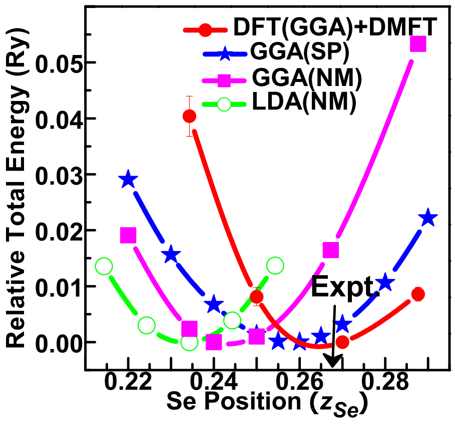


FIG. 2. (Color online). Relative total energy calculated in LDA(non-magnetic), GGA(both nonmagnetic and checkerboard spin-polarized), and DFT-DMFT methods; arrow indicates the experimental value of $z_{Se}$.

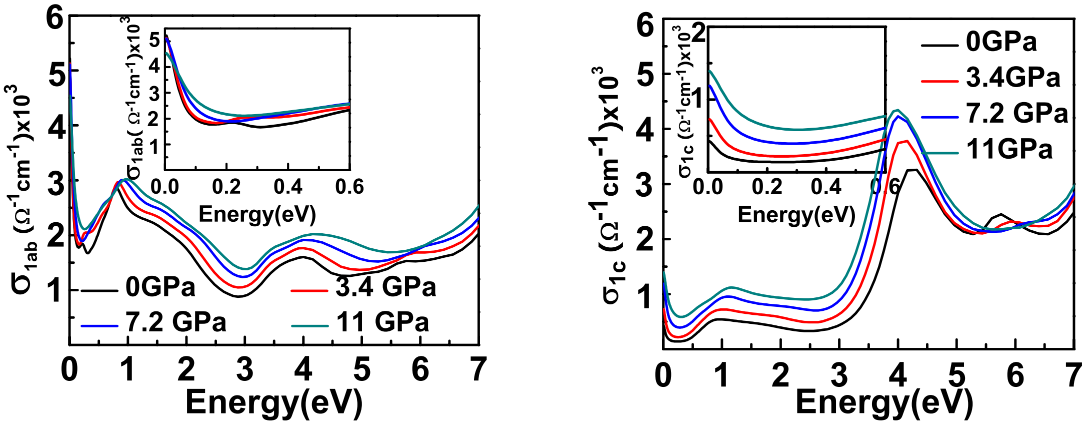


FIG. 3. (Color online). Pressure dependence optical properties at room temperature: Real part of the optical conductivity (a) along *ab*-plane and (b) along *c*-axis.

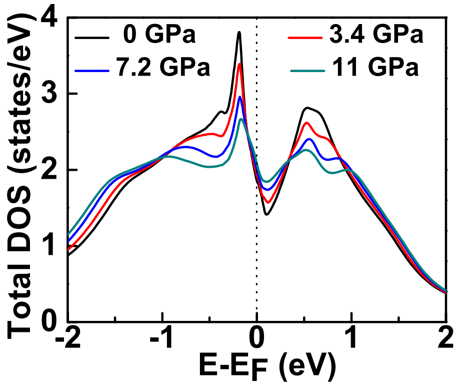


FIG. 4. (Color online). Electron density of states as a function of pressure.

TABLE I. DFT-DMFT Band-resolved deformation potential for different pressures

| Pressure (GPa) | pocket | $\mathcal{D}^{m}$ (eV/Å) | $\mathcal{D}^{avg}$(eV/Å) | $N_{kF}$ | $\mathcal{D}^{avg}_{FS}$ (eV/Å) |
|---|---|---|---|---|---|
| | h1 | 3.044 | 2.396 | 180 | |
| | h2 | 0.868 | 0.694 | 688 | |
| -2 | h3 | 0.402 | 0.382 | 884 | 0.8186 |
| | e1 | 1.585 | 0.904 | 456 | |
| | e2 | 1.405 | 1.112 | 504 | |
| | h1 | 4.439 | 4.358 | 16 | |
| | h2 | 1.342 | 1.0321 | 632 | |
| 0 | h3 | 0.268 | 0.242 | 1088 | 0.844 |
| | e1 | 1.971 | 1.291 | 616 | |
| | e2 | 1.616 | 1.282 | 468 | |
| | h1 | 4.70 | 4.199 | 16 | |
| | h2 | 1.926 | 1.394 | 724 | |
| 1.4 | h3 | 2.820 | 0.169 | 840 | 1.035 |
| | e1 | 2.198 | 1.439 | 648 | |
| | e2 | 1.729 | 1.346 | 500 | |
| | h1 | 4.844 | 3.902 | 76 | |
| | h2 | 1.381 | 1.087 | 584 | |
| 2.6 | h3 | 0.271 | 0.239 | 1004 | 0.961 |
| | e1 | 2.09 | 1.353 | 608 | |
| | e2 | 1.729 | 1.340 | 500 | |
| | h2 | 1.856 | 1.299 | 736 | |
| | h3 | 1.821 | 0.153 | 804 | |
| 3.4 | e1 | 2.390 | 1.566 | 648 | 1.027 |
| | e2 | 1.729 | 1.345 | 484 | |
| | h2 | 1.629 | 1.164 | 780 | |
| | h3 | 1.585 | 0.234 | 772 | |
| 7.2 | e1 | 2.35 | 1.469 | 728 | 0.984 |
| | e2 | 1.642 | 1.157 | 476 | |
| | h2 | 1.334 | 0.949 | 764 | |
| | h3 | 1.349 | 0.352 | 860 | |
| 11 | e1 | 2.114 | 1.352 | 816 | 0.885 |
| | e2 | 1.389 | 0.941 | 512 | |


[1] G. Kotliar, S. Y. Savrasov, K. Haule, V. S. Oudovenko, O. Parcollet, and C. A. Marianetti, Rev. Mod. Phys. **78**, 865 (2006).

[2] K. Haule, C.-H. Yee, and K. Kim, Phys. Rev. B **81**, 195107 (2010).

[3] Z. P. Yin, K. Haule, and G. Kotliar, Nat. Mater. **10**, 932 (2011).

[4] P. Blaha, K. Schwarz, G. Madsen, D. Kvasnicka, and J. Luitz, *An augmented plane wave plus local orbitals program for calculating crystal properties*, edited by K. Schwarz (Vienna University of Technology, Austria, 2001, 2001).

[5] A. Kutepov, K. Haule, S. Y. Savrasov, and G. Kotliar, Phys. Rev. B **82**, 045105 (2010).

[6] R. S. Kumar, Y. Zhang, S. Sinogeikin, Y. Xiao, S. Kumar, P. Chow, A. L. Cornelius, and C. Chen, J. Phys. Chem. B **114**, 12597 (2010).

[7] Z. P. Yin, A. Kutepov, and G. Kotliar, Phys. Rev. X **3**, 021011 (2013).

[8] J. N. Millican, D. Phelan, E. L. Thomas, J. B. Leo, and E. Carpenter, Solid State Commun. **149**, 707 (2009).

[9] D. Phelan, J. N. Millican, E. L. Thomas, J. B. Leão, Y. Qiu, and R. Paul, Phys. Rev. B **79**, 014519 (2009).

[10] S. Margadonna, Y. Takabayashi, Y. Ohishi, Y. Mizuguchi, Y. Takano, T. Kagayama, T. Nakagawa, M. Takata, and K. Prassides, Phys. Rev. B **80**, 064506 (2009).

[11] A. Subedi, L. Zhang, D. Singh, and M. Du, Phys. Rev. B **78**, 134514 (2008).

[12] A. Ciechana, M. Winiarskib, and M. Samsel-Czekaaab, Ac. Phy. Pol. A , 1 (2012).
